# Supplementary material for: Generator-Refiner-Examiner: A Tri-Module Data Augmentation Framework for 3D Human Avatar Learning from Monocular Videos
Source: arXiv:2605.23555 source file (2026-05-22)
Supplement: Supplementary file 1 [file X_suppl.tex]

% \clearpage
\setcounter{page}{1}
\maketitlesupplementary

\section{Implementation Details}
\myparagraph{Training of Refiner} For our Refiner, the diffusion UNet is initialized with the pre-trained model from the work~\cite{wu2025difix3d}. For these training images (coarse frames and GT frames), we will first crop the bounding box of the human body based on the mask, extend it outward by 0.2, and then resize it to a size of 840 * 400. When incorporating the Refiner into our framework for online improvement, we will also perform the same operation. The X-humans~\cite{shen2023xavatar} dataset has several video clips for each subject, with each clip providing approximately 100 video frames. Therefore, when selecting $T$ and $T+k$, we randomly choose $k$ within the range of (-15, 15).  For each subject in the X-Humans dataset, we will first use the basic model of ExAvatar~\cite{moon2024exavatar} for per-subject optimization. After the optimization is completed, we will use this trained model for inference and obtain coarse frames. In the Refiner training, the final training loss of geometry learning consists of three parts, L1, LPIPS, and SSIM losses ($\mathcal{L}_{1}$, $\mathcal{L}_{SSIM}$, $\mathcal{L}_{LPIPS}$):
\begin{equation} \label{equafinal}
    \mathcal{L} = \mathcal{L}_{1} + \alpha \cdot \mathcal{L}_{SSIM} + \beta \cdot \mathcal{L}_{LPIPS},
\end{equation}
where $\alpha$ and $\beta$ are hyperparameters that control the strength, with $\alpha=0.2$ and $\beta=0.2$. This loss will be used for reconstructing the GT frame at time $T$, the SMPL normal map at time $T$, and the GT frame at time $T+k$. The number of timesteps is 200. We utilized 4 A6000 GPUs for parallel training, setting the batch size to 1, and trained for three days.

\myparagraph{Training of Examiner} For our Examiner, the ViT is initialized with the pre-trained model from the work~\cite{caron2021emerging}, the base model with a patch size of 8 and an image size of 224. For these training images (coarse frames and GT frames), we adopt the same preprocessing operation as in the training of the Refiner. We add an extra operation to randomly crop a region of size 224 * 224 from the image of size 840 * 400. The value of $k$ is also in the range (-15, 15). The number of blocks in the Examiner is 2, with the $C^1$ of the first block having a size of 768, and the $C^2$ of the second block having a corresponding size of 384. 

\myparagraph{Training of the monocular video reconstruction } Once we have prepared our trained Refiner and Examiner, we can begin training and fine-tuning our baseline model of monocular video 3D human reconstruction. We first deploy our Generator, setting up a separate branch to synthesize new samples. In this branch, we first obtain perturbations by sampling from a Gaussian distribution. For the SMPL pose, we set that each parameter perturbation $\Delta \theta_i$ is sampled from the Gaussian distribution $N_i(\mu, \Sigma)$, where the mean $\mu$ is set to 0 and the variance $\Sigma$ is set to 0.03. Finally, we use the clamp function to restrict the sampled values to the range of -1 to 1 to avoid possible extreme values. The camera angles, azimuth, and elevation are set to fluctuate according to a Gaussian distribution with a mean of 0 and a variance of 3. These new parameters are fed into the frozen baseline model and rendered to obtain a coarse human image with a new pose and viewpoint. This image, along with the original ground truth (GT) frame and the SMPL normal map rendered from the new SMPL pose, is fed into our prepared Refiner model for refinement, resulting in a refined image. Subsequently, this refined image, together with the original GT frame, is fed into our Examiner for scoring. The selected refined image will be considered as a pseudo GT frame and used in a regular model training process. We set the probability of using the pseudo GT frame for training equal to the probability of using the original GT frame for training.
We employ our augmentation strategy in the last epoch when the original model has already converged, and we introduce augmented samples for fine-tuning.

\section{Dataset}

We conduct experiments on two publicly available datasets to evaluate the performance of our method, aligning with the experimental setup of the original work~\cite{moon2024exavatar}.

\myparagraph{X-Humans~\cite{shen2023xavatar}} X-Humans is a captured dataset that provides high-quality 3D scans and RGBD videos of multiple human subjects. Compared to NeuMan, this dataset offers richer variations in facial expressions and hand poses, making it suitable for evaluating the expressiveness of whole-body avatars. Two experimental protocols are supported by the dataset: one using 3D scans and another using RGBD images for avatar creation. Following ExAvatar~\cite{moon2024exavatar}, we only leverage monocular RGB videos (without depth information) and compare our results against some method~\cite{shen2023xavatar} that uses RGBD data. Same as ~\cite{moon2024exavatar}, we use three subjects (0028, 0034, and 0087) for evaluation, as their pre-trained models under the RGBD protocol are publicly accessible. We strictly follow the official training and testing splits to maintain consistency with previous evaluations.

\begin{table*}%[!t]
\begin{center}
    \caption{\textbf{Comparisons of the training time of different methods.}}\label{training_time}
\scalebox{1}{
\begin{tabular}
{l|cccccc}
\toprule

{-}  & {GaussianAvatar} & {Vid2Avatar} & {NeuMan}  & {EVA} & {ExAvatar} & {Ours}\\
% & PSNR $\uparrow$ & SSIM $\uparrow$ & LPIPS $\downarrow$  & PSNR $\uparrow$ & SSIM $\uparrow$ & LPIPS $\downarrow$  & PSNR $\uparrow$ & SSIM $\uparrow$ & LPIPS $\downarrow$ \\

\midrule%\&JLA
     {Training time} & 1 Days & 1.5 Days & 3 Days & 2 Hours & 5 Hours & 5.5 Hours \\

\bottomrule
    \end{tabular}
}
    		% \vspace{-0.2cm}

    		% \vspace{-0.6cm}

\end{center}
\end{table*}

\begin{table}%[!t]
\begin{center}
\caption{\textbf{Module ablation study.} We compare our proposed Refiner module with a general scene Refiner \cite{wu2025difix3d} through ablation experiments.\label{exp_abl_scene}}
    		% \vspace{-0.8cm}
    		% \vspace{-0.7cm}
\scalebox{0.72}{
\begin{tabular}
{l|ccc}
\toprule

\multirow{2}{*}{Methods}  & \multicolumn{3}{c}{00028}  \\
& PSNR $\uparrow$ & SSIM $\uparrow$ & LPIPS $\downarrow$  \\

\midrule%\&JLA
     Baseline  & 30.5842 & 0.9814 & 0.0181 \\  
+ Generator & 31.2905 & 0.9825 & 0.0170 \\ 
+ Generator\&Refiner(~\cite{wu2025difix3d}) & 31.1819 & 0.9822 & 0.0172 \\ 
+ Generator\&Refiner(Ours) & \textbf{32.6586} & \textbf{0.9847} & \textbf{0.0146}\\    
% + Generator\&Refiner\&Examiner & \textbf{33.0412} & \textbf{0.9851} & \textbf{0.0143} \\    

\midrule

& \multicolumn{3}{c}{00034} \\
% & PSNR $\uparrow$ & SSIM $\uparrow$ & LPIPS $\downarrow$  \\

\midrule
%\&JLA
     Baseline   & 28.7533 & 0.9659 &  0.0292\\  
+ Generator & 28.9654  & 0.9665 &  0.0280\\ 
+ Generator\&Refiner(~\cite{wu2025difix3d}) & 28.8542 & 0.9663 & 0.0283 \\ 
+ Generator\&Refiner(Ours) & \textbf{29.6413} & \textbf{0.9678} & \textbf{0.0263} \\    
% + Generator\&Refiner\&Examiner & \textbf{29.8745} & \textbf{0.9681} & \textbf{0.0261}\\    
\bottomrule
    \end{tabular}
}
    		% \vspace{-0.2cm}

\end{center}
\end{table}

\begin{table}%[!t]
\begin{center}

\caption{\textbf{Ablation study about the $\Sigma$ in Generator}\label{exp_abl_Sigma}}
    		% \vspace{-0.8cm}
\scalebox{0.8}{
\begin{tabular}
{l|ccc}
\toprule

\multirow{2}{*}{Methods}  & \multicolumn{3}{c}{00028}  \\
& PSNR $\uparrow$ & SSIM $\uparrow$ & LPIPS $\downarrow$  \\

\midrule%\&JLA
$\Sigma$ = 0.03 & \textbf{33.0412} & \textbf{0.9851} & \textbf{0.0143} \\    
$\Sigma$ = 0.01 & 32.8522 & 0.9846 & 0.0147 \\    
$\Sigma$ = 0.05 & 32.9488 & 0.9848 & 0.0146 \\    

\midrule

    \end{tabular}
}
    		% \vspace{-0.2cm}

    		% \vspace{-0.7cm}

\end{center}
\end{table}

\myparagraph{NeuMan~\cite{jiang2022neuman}} The NeuMan dataset comprises multiple short monocular videos captured in unconstrained real-world scenarios. Each video features a single individual engaged in natural movements (e.g., walking) for approximately 15 seconds. Following the selection criteria of prior studies~\cite{moon2024exavatar}, we utilize four representative video sequences—bike, citron, jogging, and seattle—due to their comprehensive coverage of human body regions and minimal motion blur. We adhere to the official training and testing partition provided by the dataset to ensure fair comparison with existing methods.

\section{More Experiments} 

% In Table~\ref{exp_abl_Sigma}, we perform an ablation study on the $\Sigma$ parameter in the Generator. Our experiments reveal that when $\Sigma$ is set to 0.03, the best results are achieved. This is because when the value of $\Sigma$ is small, the new poses generated have little difference from the original poses, resulting in minimal changes and insufficient augmentation. On the other hand, when $\Sigma$ is too large, the generated poses differ significantly from the original ones, leading to the creation of many unreasonable human poses, such as hands entering the body, as shown in Figure~\ref{fig: Value_of_examiner}. Introducing such samples can harm the model's performance.

In Table~\ref{training_time}, we compare the training efficiency of various monocular 3D human reconstruction methods. ExAvatar demonstrates considerable speed advantages over GaussianAvatar, Vid2Avatar, and NeuMan. While EVA achieves marginally faster training, our method incurs a modest increase in training time compared to ExAvatar—attributed to the integration of our tri-module data augmentation pipeline (Generator, Refiner, Examiner) that enriches training data and enhances reconstruction fidelity. This trade-off between computational cost and performance gain is well-justified, as our method delivers superior reconstruction quality across key metrics (PSNR, SSIM, LPIPS) on both X-Humans and NeuMan datasets.

In Table \ref{exp_abl_scene}, it is found that when the general-purpose scene Refiner \cite{wu2025difix3d} is directly applied to human-centric data, its performance is slightly lower than that of the Generator-only setup. A possible reason for this phenomenon lies in the adaptability of the method itself: while such general-purpose refiners work well for common objects in scenes (e.g., indoor decorations, outdoor landscapes), they cannot be directly applied to human targets. Unlike general objects that only require ensuring overall consistency (e.g., harmony of background lighting), human bodies have more special texture details (e.g., skin texture) and geometric structures (e.g., body contours, wrinkles in clothes). The general Refiner, optimized for common objects, lacks targeted design for these human-specific features.

In Table~\ref{exp_abl_Sigma}, we perform ablation on the $\Sigma$ parameter in the generator. Our experiments found that when the value of $\Sigma$ is 0.03, the best results can be achieved. This is because when the value of $\Sigma$ is small, the new pose generated does not differ much from the original pose, resulting in minimal change and insufficient augmentation. Conversely, when the value of $\Sigma$ is too large, the generated pose deviates significantly from the original pose, leading to many unreasonable human poses, such as the hand entering the body, as illustrated in Figure~\ref{fig: Value_of_examiner}. This results in some texture color errors. Introducing such samples will harm the model's performance.

\section{More Visualization} 

To further validate the effectiveness of the Examiner module, we visualize its quality scoring and filtering performance in Figure~\ref{fig: Value_of_examiner}. In the figure, the Examiner assigns distinct scores to refined images based on their detail consistency with the GT frame. Refined images suffering from subtle flaws, such as inconsistent texture or distorted local geometry, are given lower scores. In contrast, high-quality refined images that preserve authentic texture details receive higher scores. This demonstrates the Examiner’s filtering ability: it effectively distinguishes between valid and flawed samples by quantifying detail-level similarity, ensuring only high-fidelity refined images are retained as pseudo-GT. Such selective sampling avoids introducing noisy data into the training process, contributing to the final reconstruction accuracy of our 3D avatar model.

\begin{figure*}
    \centering
    \includegraphics[width=1.0\linewidth]{figs/Value_of_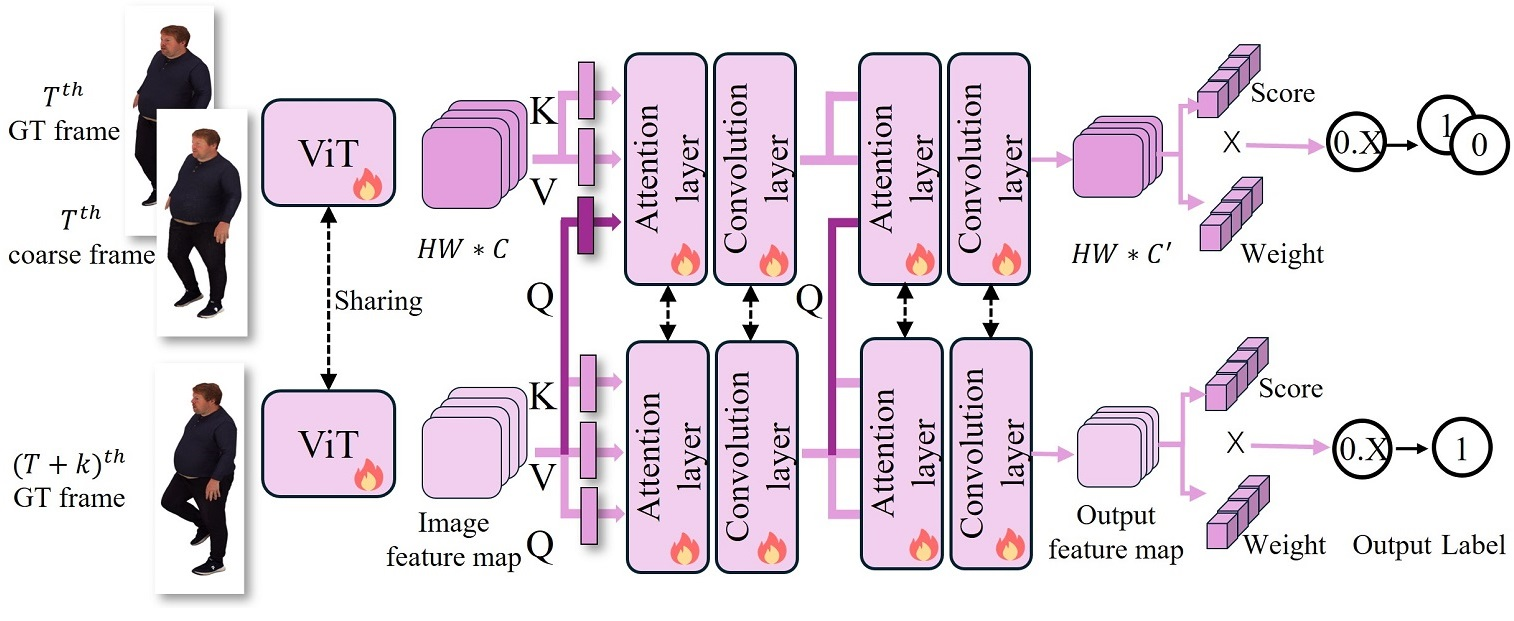}
    % \vspace{-0.6cm}
    \caption{\textbf{Examiner scores the refined images differently.} ``Source GT frame" is for grasping the pose and texture of the human in the original video frame. From this original frame(pose), we use our Generator and Refiner to obtain two different refined images, 1 and 2 (in different poses), and then use the Examiner to score them (Examiner takes refined image and source GT frame as input to output the similarity value).  It is observed that the Examiner exhibits a filtering effect: refined images with subtle flaws, such as inconsistent texture compared to the GT frame, receive lower scores. This filtering mechanism is key to the Examiner’s contribution to performance improvement: by quantifying detail-level similarity, the Examiner effectively screens out low-fidelity samples and retains only those refined images that align more closely with the real-world characteristics of the GT frame.  } 
    \label{fig: Value_of_examiner}
    % \vspace{-0.1cm}
\end{figure*}

To further supplement the qualitative evidence for the effectiveness of our Refiner, Figures \ref{fig: more_refined_1} and \ref{fig: more_refined_2} present additional visual comparisons between images generated by our Generator and those refined by our subsequent Refiner. As can be observed from the displayed samples, the Refiner enhances the quality of human content in key aspects. Specifically, for human details that are critical to overall fidelity, such as subtle skin texture, clear clothing folds, the Refiner effectively reduces slight blurriness or inconsistency present in the generated images, making these details more realistic and natural. Meanwhile, the Refiner maintains the overall naturalness of the image content, avoiding unnatural visual artifacts. This qualitative improvement is consistent with the quantitative gains reflected in previous ablation experiments, further confirming that our Refiner can target and enhance fine-grained quality

\begin{figure*}
    \centering
    \includegraphics[width=1.0\linewidth]{figs/more_refined_1.jpg}
    % \vspace{-0.6cm}
    \caption{\textbf{Display of the generated images from Generator and refined images from Refiner.} We present additional qualitative results to visually demonstrate the difference between images generated by our Generator and those further refined by our Refiner. Specifically, it is found that these samples present improvements in human details and overall visual fidelity after refinement. These results further verify that our Refiner can effectively enhance the fine-grained quality of different human regions while maintaining the naturalness of the generated content. }
    \label{fig: more_refined_1}
    % \vspace{-0.1cm}
\end{figure*}

\begin{figure*}
    \centering
    \includegraphics[width=1.0\linewidth]{figs/more_refined_2.jpg}
    % \vspace{-0.6cm}
    \caption{\textbf{Display of the generated images from Generator and refined images from Refiner.} We present additional qualitative results to visually demonstrate the difference between images generated by our Generator and those further refined by our Refiner. Specifically, the displayed samples focus on highlighting improvements in human details and overall visual fidelity after refinement. These results further verify that our Refiner can effectively enhance the fine-grained quality of human-related regions while maintaining the naturalness of the generated content.. } 
    \label{fig: more_refined_2}
    % \vspace{-0.1cm}
\end{figure*}

To further validate the reconstruction ability of our method on unseen poses— a key challenge in monocular 3D human avatar reconstruction—we conduct additional experiments using novel poses. These novel poses are generated by applying Gaussian perturbations to the poses of the original set of X-Humans and NeuMan (consistent with the Generator’s sampling strategy), resulting in movements that are different from the original data distribution (e.g., wider leg stances, dramatic neck twists, and expansive body movements) and introduce greater reconstruction difficulty.
As shown in Figures~\ref{fig: Novel_pose1} and \ref{fig: Novel_pose2}, ExAvatar exhibits noticeable artifacts under these novel poses, such as geometric breakage, unnatural texture inconsistencies, and abnormal spots. In contrast, our method effectively mitigates these issues, achieving better structural integrity and texture consistency across these novel poses. Extending the validation to additional subjects (Figure~\ref{fig: Novel_pose3}) confirms this trend.
These results underscore the value of our tri-module framework: by enriching training with diverse pose variations and ensuring high-fidelity pseudo-GT, our method overcomes the baseline’s limitations from limited training data diversity, enabling robust handling of novel poses.

\begin{figure*}
    \centering
    \includegraphics[width=1.0\linewidth]{figs/Novel_pose1.jpg}
    % \vspace{-0.6cm}
    \caption{\textbf{Comparative advantages of our method in more novel poses.}  To show the advantages of our model relative to ExAvatar, the strongest SOTA method, we derived some novel poses not originally present in the dataset by applying Gaussian perturbations to the poses in the test set. These postures may not conform to the original distribution in the dataset, and may present more difficulty in certain movements compared to the originals. Since the novel pose presented does not exist in the original dataset, we here provide an adjacent ``real frame" as a reference. We then show the results rendered from the 3D avatars reconstructed from ExAvatar and our method under the same poses and cameras. It is found that ExAvatar's deficiencies become more apparent with these new poses. For instance, in the top-left case, when the human's legs are spread widely, some breakage occurs, whereas our model does not exhibit this issue. Similarly, in the top-right and bottom-right cases, when the neck of the human twists dramatically, ExAvatar produces noticeable and unnatural artifacts. Additionally, in the bottom-left example, when the human body twists considerably, unnatural artifacts appear on the clothing's texture. In contrast, our method greatly improves upon these issues.}
    \label{fig: Novel_pose1}
    % \vspace{-0.1cm}
\end{figure*}

\begin{figure*}
    \centering
    \includegraphics[width=1.0\linewidth]{figs/Novel_pose2.jpg}
    % \vspace{-0.6cm}
    \caption{\textbf{Comparative advantages of our method in more novel poses.} To show the advantages of our model relative to ExAvatar, the strongest SOTA method, we derived some novel poses not originally present in the dataset by applying Gaussian perturbations to the poses in the test set. These postures may not conform to the original distribution in the dataset and may present more difficulty in certain movements compared to the originals. It is found that ExAvatar's deficiencies become more apparent with these new poses. For instance, in the top-left case, when the character's movements become more expansive, the artifacts at the edges of the clothing become significantly more pronounced. In the top-right and bottom-left cases, under certain specific poses, the ExAvatar model reconstructs the character's arms with white artifacts, and there are red artifacts at the seams of the clothing. In the bottom-right case, the head of the character reconstructed by ExAvatar exhibits abnormal spots. However, with the improvements in our method, these deficiencies are greatly mitigated. } 
    \label{fig: Novel_pose2}
    % \vspace{-0.1cm}
\end{figure*}

\begin{figure*}
    \centering
    \includegraphics[width=1.0\linewidth]{figs/Novel_pose3.jpg}
    % \vspace{-0.6cm}
\caption{\textbf{Comparative advantages of our method on other subjects with novel poses.} Similarly, we derived some new poses not present in the dataset for other subjects to compare the advantages of our method relative to ExAvatar. It is found that ExAvatar exhibits artifacts in these new poses. In contrast, after the introduction of our method, these issues showed great improvement, demonstrating that our approach can indeed achieve better results on certain novel poses, even in these more open postures.}   \label{fig: Novel_pose3}
    % \vspace{-0.1cm}
\end{figure*}

% to 512x512 pixels and the Fourier expansion order ($q$) to 8. During training, we render human scans online using the official nvdiffrast library. We randomly sample 8 views to generate 8 RGB images, which are used to constrain the proposed Gaussian, and we then select one of these images as the input view, whose camera elevation and azimuth are set to 0,0. Note that we sample the front views at random elevation and azimuth. We only set/assume these degrees of the front view all to zero, to normalize other views. The learning rate for the AdamW~\cite{adamw} optimizer is set to  $5\times10^{-5}$. In training, we use the officially released fitting SMPL-X parameters~\cite{tao2021function4d_thuman} as input and the default disturbance value ($\alpha$) is set to 0.25. The pre-trained UNet of the wrinkle-level refinement module is from the work~\cite{unique3d}. Specifically, we freeze the VAE and CLIP image encoder and only update the UNet. All of the input images are rendered with nvdiffrast and resized to 512x512 pixels. We randomly selected 8 horizontal camera-rendered images and top and bottom camera-rendered images as our initialization inputs and de-noising conditions. During training, we set the de-noising step $k$ to 1. The learning rate of AdamW optimizer is set to $1\times10^{-5}$. All models are trained to converge.
